# Supplementary material for: Properties with Holes: Meta-Property-Based Testing of Data-Intensive Computing Frameworks
Source: arXiv:2606.11132 source file (2026-10-20)
Supplement: Supplementary file 1 [file appendix.tex]

\section*{Appendix A: Proof on cutoff property}

\paragraph{Cutoff Aggregation.}
The cutoff aggregation returns the smallest threshold \(v\) such that at most
a \(p\)-fraction of values are greater than or equal to \(v\). Intuitively,
it identifies a threshold above which only a small fraction of values remain.

Formally, let the value domain be the extended real numbers
\(\mathbb{R}\cup\{-\infty,+\infty\}\). Given a multiset \(X\) and a fraction
\(p\in[0,1]\), define
\[
\mathrm{cutoff}(X,p)
=
\inf
\left\{
v
\;\middle|\;
|\{x\in X \mid x\ge v\}|
\le p|X|
\right\}.
\]

\paragraph{Example.}
Consider two classes of student scores. Class \(A\) contains the scores
\[
X_A=\{91,92,\ldots,100\},
\]
while class \(B\) contains
\[
X_B=\{81,82,\ldots,90\}.
\]
Suppose we set \(p=0.1\), meaning that the cutoff identifies a threshold above
which at most the top \(10\%\) of scores remain.

For class \(A\), we have \(p|X_A|=1\). Observe that for every
\(\varepsilon>0\), exactly one value (\(100\)) is greater than or equal to
\(99+\varepsilon\), so every \(99+\varepsilon\) satisfies the cutoff
condition. However, exactly two values (\(99\) and \(100\)) are greater than
or equal to \(99\), so \(99\) itself does not satisfy the condition. Hence
the set of valid thresholds is \((99,+\infty]\), whose infimum is \(99\).
Therefore,
\[
\mathrm{cutoff}(X_A,0.1)=99.
\]

Similarly,
\[
\mathrm{cutoff}(X_B,0.1)=89.
\]

Now consider the full dataset \(X=X_A\uplus X_B\). Since \(|X|=20\), we have
\(p|X|=2\). For every \(\varepsilon>0\), exactly two values (\(99\) and
\(100\)) are greater than or equal to \(98+\varepsilon\), so every
\(98+\varepsilon\) satisfies the cutoff condition. However, three values
(\(98\), \(99\), and \(100\)) are greater than or equal to \(98\), so \(98\)
itself does not satisfy the condition. Hence,
\[
\mathrm{cutoff}(X,0.1)=98.
\]

\paragraph{Boundary Case and Well-Definedness.}
When \(X=\emptyset\), we have
\(
|\{x\in X \mid x\ge v\}| = 0
\)
and
\(
p|X|=0
\)
for every \(v\). Hence every threshold satisfies the cutoff condition. Since
the value domain includes \(-\infty\), the infimum of all valid thresholds
exists and equals
\[
\mathrm{cutoff}(\emptyset,p)=-\infty.
\]
Therefore, \(\mathrm{cutoff}(X,p)\) is well-defined for all multisets \(X\).

\paragraph{Property.}
Suppose \(X=\biguplus_{i=1}^m X_i\) is a partition of \(X\). Then
\[
\mathrm{cutoff}(X,p)
\ge
\min_i \mathrm{cutoff}(X_i,p).
\]

Intuitively, the global cutoff cannot be smaller than every local cutoff.
Otherwise, each partition would already contain more than a \(p\)-fraction of
values above that threshold, which would imply that the full dataset also
violates the cutoff condition.

\begin{proof}
Let
\(
v^*=\min_i \mathrm{cutoff}(X_i,p).
\)
We show that
\(
\mathrm{cutoff}(X,p)\ge v^*.
\)

Consider any \(v<v^*\). Since \(v^*\) is the minimum local cutoff, we have
\(
v<\mathrm{cutoff}(X_i,p)
\)
for every partition \(X_i\). By the definition of cutoff, this implies that
\(v\) cannot satisfy the cutoff condition for \(X_i\). Therefore,
\[
|\{x\in X_i \mid x\ge v\}| > p|X_i|.
\]

Summing over all partitions gives
\[
\sum_i |\{x\in X_i \mid x\ge v\}|
>
\sum_i p|X_i|
=
p|X|.
\]

Since the \(X_i\)'s form a disjoint partition of \(X\),
\[
|\{x\in X \mid x\ge v\}|
>
p|X|.
\]

Hence \(v\) does not satisfy the cutoff condition for \(X\). Since this holds
for every \(v<v^*\), no value smaller than \(v^*\) can belong to the valid
threshold set for \(X\). Therefore,
\[
\mathrm{cutoff}(X,p)\ge v^*.
\]
\end{proof}

\paragraph{Intuition from the Example.}
In the example above, the local cutoffs are \(99\) and \(89\), while the
global cutoff is \(98\). Therefore,
\[
98 \ge \min\{99,89\}=89.
\]
This matches the theorem: once a threshold becomes smaller than the minimum
local cutoff, every partition would already contribute too many values above
that threshold, forcing the global dataset to violate the cutoff condition as
well.
